# Supplementary material for: Orion: A Unified Visual Agent for Multimodal Perception, Advanced Visual Reasoning and Execution
Source: arXiv:2511.14210 source file (2025-11-19)
Supplement: Supplementary file 1 [file 1_evaluation_additional_details.tex]

\subsection{Evaluation additional details}
\label{sub:appendix:quantitative_evaluation}

Please see a description of the benchmarks considered, along with details of how scores in the main text were obtained in Table~\ref{tab:benchmark_descriptions}.

{\small
    
    \begin{longtable}{p{0.15\textwidth} p{0.35\textwidth} p{0.4\textwidth}}
    
    \toprule
    \textbf{Benchmark} & \textbf{Description} & \textbf{Details} \\
    \midrule
    \endfirsthead
    
    \toprule
    \textbf{Benchmark} & \textbf{Description}  & \textbf{Details} \\
    \midrule
    \endhead
    
    \midrule
    \multicolumn{3}{r@{}}{Continued on next page} \\
    \endfoot
    
    \bottomrule
    \addlinespace[10pt]
    \caption{Description of the benchmarks used, along with extra details about subsets, variants and model specifications.}
    \label{tab:benchmark_descriptions} \\ 
    \endlastfoot

%%% CODE
    LiveCodeBench & Code generation in Python \cite{jain2024livecodebenchholisticcontaminationfree}. & Results are taken from \url{https://livecodebench.github.io/leaderboard.html} (1/1/2025 - 5/1/2025 in the UI) or, where not available, run internally by us. For Section~\ref{sub:thinking} and Figure~\ref{fig:thinking_budget_model} and \ref{fig:thinking_budget}, results are calculated on the version of the eval corresponding to  10/05/2024 - 01/04/2025 in the UI, and are based on internal results. \\
    \midrule
    
    Aider Polyglot & Code editing in C++, Go, Java, JavaScript Python and Rust \cite{aider_leaderboard}. See \url{https://aider.chat/2024/12/21/polyglot.html#the-polyglot-benchmark} for a full description of this task. & We report results on the ``diff'' or ``diff-fenced'' edit format (see \url{https://aider.chat/docs/more/edit-formats.html} for a description of the different formats). The score reported are the pass rate average of 3 trials. Numbers come from \url{https://aider.chat/docs/leaderboards/}\\
    \midrule
    
    SWE-bench Verified & Agentic coding: evaluates AI agents on real-world programming tasks from GitHub \cite{jimenez2024swebench, chowdhury2024swebenchverified}. & Gemini uses an internal agentic harness equipped with tools to navigate the repo, edit files, and test the code. \par We report scores for two modes: performance of a single agentic trace (``single attempt''), and performance of a scaffold that samples multiple agentic traces and re-reranks them before evaluation using Gemini's own judgement (``multiple attempts''). \par All evaluations are done with temperature=1, topp=0.99, topk=1024. \\
    \midrule

%%% REASONING
    GPQA \par (diamond) & Challenging dataset of questions written by domain experts in biology, physics, and chemistry \cite{rein2024gpqa}. & \\
    \midrule
    
    Humanity’s Last Exam & Challenging dataset of questions written by domain experts in a wide range of disciplines, including mathematics, physics, chemistry, biology and computer science \cite{phan2025_hle_humanity_last_exam_paper}. & No tool use variant.
    \par Reported results are from \url{https://scale.com/leaderboard/humanitys_last_exam}.
    \par For DeepSeek they are taken from \url{https://scale.com/leaderboard/humanitys_last_exam_text_only} (leaderboard for performance on the text-only questions) and in the case of the Gemini 2.0 models, these results are on an earlier HLE dataset, obtained from \url{https://scale.com/leaderboard/humanitys_last_exam_preview} (indicated with a $\dagger$ in Table~\ref{tab:results_gemini})    
    \\
    \midrule

%%% FACTUALITY
    SimpleQA & World knowledge factuality with no search enabled \cite{wei2024measuring_simpleqa}. & F1 scores are obtained from \url{https://github.com/openai/simple-evals} and, where not available, run internally by us. \\
    \midrule
    
    FACTS Grounding & Ability to provide factually correct responses given documents and diverse user requests. \cite{jacovi2025factsgrounding} & Results are sourced from \url{https://www.kaggle.com/benchmarks/google/facts-grounding} \\
    \midrule
    
%%% MULTILINGUALITY
    Global MMLU (Lite) & MMLU translated by human translators into 15 languages. \cite{singh2024globalmmluunderstandingaddressing} & The lite version includes 200 Culturally Sensitive and 200 Culturally Agnostic samples per language, see \url{https://huggingface.co/datasets/CohereLabs/Global-MMLU-Lite} \\
    \midrule
    
    ECLeKTic & A closed-book QA dataset that evaluates cross-lingual knowledge transfer \cite{goldman2025eclekticnovelchallengeset}. & \\
    \midrule
    
%%% MATH
    AIME 2025 & Performance on 30 questions from American Invitational Mathematics Examination from 2025 \cite{balunovic2025matharenaevaluatingllmsuncontaminated}. & Results are sourced from \url{https://matharena.ai/}.\\
    \midrule
    
    HiddenMath-Hard & Competition-level math problems, Held out dataset AIME/AMC-like, crafted by experts and not leaked on the web. & \\
    \midrule

%%% LONG-CONTEXT
    LOFT (hard retrieval subset) & Long context multi-hop and multi-needle retrieval evaluation of 300 queries \cite{lee2024can_loft}. & We report the results on two variants: an up to 128K average context length variant to ensure they can be comparable with other models and a pointwise value for 1M context window to show the capability of the model at full length.  \\
    \midrule
    
    MRCR-V2 (8-needle) & MRCR-V2 is a significantly harder instance of the MRCR family of long-context evaluations \cite{vodrahalli2024michelangelo_mrcr_v2}. Compared to MRCR-V1, we increase the nesting of the dictionary size to depth 3 rather than 2 by including a style parameter (for instance, an example key might be ``write a poem about penguins in an archaic style'', rather than just ``write a poem about penguins''). & The methodology has changed compared to previously published results: we focus on a harder, 8-needle version (compared to the 4-needle version used before). 
    \par We report the results on two variants: an up to 128K average context length variant to ensure they can be comparable with other models and a pointwise value for 1M context window to show the capability of the model at full length. 
    \\
    \midrule

%%% IMAGE UNDERSTANDING
    MMMU & Multi-discipline college-level multimodal image understanding and reasoning problems. \cite{yue2024mmmu} & \\
    \midrule

    Vibe-Eval (Reka) & Image understanding evaluation, featuring particularly challenging examples. \cite{padlewski2024vibeevalhardevaluationsuite} & Gemini is used as a judge. \\
    \midrule

    ZeroBench & Challenging image understanding evaluation that requires multi-step reasoning. \cite{roberts2025zerobench} & Gemini is used as a judge. Average over 4 runs. \\
    \midrule

    BetterChartQA & A comprehensive chart understanding evaluation that covers 9 disjoint capability buckets. The chart
images are randomly sampled from the web and QA pairs are written by professional human annotators to reflect the wide distribution
of chart styles and real-world cases. \cite{geminiteam2024gemini} & Gemini is used as a judge. \\
    \midrule

%%% AUDIO UNDERSTANDING
    FLEURS & Automatic speech recognition \cite{conneau2023fleurs}. & 0-shot queries to public APIs for all models. \par Used a subset of 53 languages (out of 102); we filtered languages for which either model responses were too incompatible to ground truth responses to be fairly scored. \par We use Word-Error-Rate WER (lower is better) except for four segmented languages where we aggregate Character-Error-Rates (Chinese, Japanese, Korean and Thai). \\
    \midrule

    CoVoST 2 & Speech to text translation \cite{wang2020covost2}. & 0-shot queries to public APIs for all models. \par We report BLEU scores for translating 21 languages to English. \\
    \midrule
    
%%% VIDEO UNDERSTANDING
    ActivityNet-QA & General video understanding \cite{activitynetqa} & Test subset, 0-shot. \par Videos were processed at 1fps and linearly subsampled to a maximum of $N_{frames}=1024$ frames. For GPT 4.1, we used 500 frames due to API limitations. \\
    \midrule
    
    EgoTempo & Egocentric video understanding \cite{plizzari2025omnia_egotempo} & Test subset, 0-shot. \par Same processing as above with $N_{frames}=256$. \\
    \midrule
    
    Perception Test & Perceptual understanding/reasoning \cite{patraucean2023perception} & Test subset, 0-shot. \par Same processing as above with $N_{frames}=256$. \\
    \midrule
    
    QVHighlights & Moment retrieval \cite{lei2021detecting_qvhighlights} & Validation subset, 4-shots. Accuracy measured with R1@0.5. \par Same processing as above with $N_{frames}=256$. \\
    \midrule
    
    VideoMMMU & Video knowledge acquisition \cite{hu2025videommmuevaluatingknowledgeacquisition} & Test subset, 0-shot. \par Same processing as above with $N_{frames}=256$. \\
    \midrule
    
    1H-VideoQA & Hour-long video understanding \cite{geminiteam2024gemini} & Test subset, 0-shot. \par Same processing as above with $N_{frames}=7200$. \\
    \midrule
    
    LVBench & Long video understanding \cite{wang2024lvbenchextremelongvideo} & Test subset, 0-shot. \par Same processing as above with $N_{frames}=1024$. \\
    \midrule
    
    VideoMME & Long video understanding \cite{fu2025videomme} & 0-shot. Audio + visual uses the Long subset of test set, audio + visual + subtitles uses full test set. \par Same processing as above with $N_{frames}=1024$. \\
    \midrule
    
    VATEX & General video captioning \cite{wang2019vatex} & Test subset, 4-shots. CIDEr score. \par Same processing as above with $N_{frames}=64$. \\
    \midrule
    
    VATEX-ZH & Chinese video captioning \cite{wang2019vatex} & Validation subset, 4-shots. CIDEr score. \par Same processing as above with $N_{frames}=64$. \\
    \midrule
    
    YouCook2 Cap & Instructional video captioning \cite{ZhXuCoAAAI18_youcook2} & Validation subset, 4-shots. CIDEr score. \par Same processing as above with $N_{frames}=256$. \\
    \midrule

    Minerva & Complex video reasoning \cite{nagrani2025minervaevaluatingcomplexvideo} &  Test subset, 0-shot. \par Same processing as above with $N_{frames}=1024$. \\
    \midrule

    Neptune & Long video understanding \cite{nagrani2025neptunelongorbitbenchmarking} & Test subset, 0-shot. \par Same processing as above with $N_{frames}=1024$. \\
    \midrule

    \end{longtable}
}
